# Supplementary material for: Semi-supervised Hypergraph Node Classification on Hypergraph Line Expansion
Source: arXiv:2005.04843 source file (2023-04-13)
Supplement: Supplementary file 1 [file appendix.tex]

\appendix

\section{Proof of Theorem~\ref{thm:bijective}} \label{proof:thm1}
\textbf{Statement of the Theorem.} \emph{Under the construction, for a hypergraph $G_H$ and its line expansion $G_l$, the mapping $f$ from hypergraph to line expansion (i.e., $\phi: G_H \rightarrow G_l$) is bijective.}

To prove the bijectivity of mapping $\phi: G_H \rightarrow G_l$, we present a graph isomorphism theorem \cite{whitney1992congruent} below. Node that the bipartite representation of hypergraph from $G_H \rightarrow G_b$ is an one-to-one mapping. $G_b$ is a graph with heterogeneous nodes. In the following, we will use $G_b$ to present $G_H$.

\begin{figure}[t]
	\centering
	\includegraphics[width=0.35\textwidth]{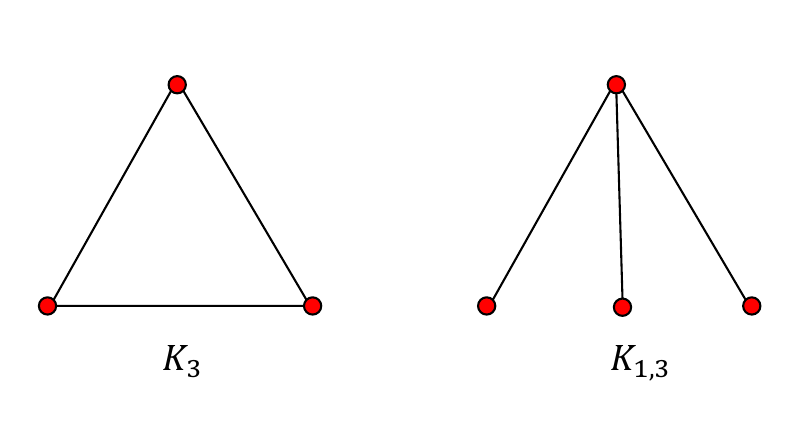}
	\vspace{-4mm}
	\caption{The Exception of Whitney's Theorem}
	\label{fig:appendix2}
\end{figure}

\begin{thm} \label{thm:whitney}
(Whitney Graph Isomorphism Theorem.) Two connected graphs are isomorphic if and only if their line graphs are isomorphic, with a single exception: $K_3$, the complete graph on three vertices, and the complete bipartite graph $K_{1,3}$, which are not isomorphic but both have $K_3$ as their line graph
\end{thm}

\begin{definition} \label{def:maximummatching}
(Maximum Independent set.) An independent set is a set of vertices in a graph, no two of which are adjacent. A maximum independent set is an independent set of largest possible size for a given graph $G$.
\end{definition}

\begin{proof}
For the bipartite representation of the hypergraph, it could be unconnected when parts of the vertices are only incident to parts of the hyperedges. In that case, we could consider it as a union of several disjoint connected components and prove them one by one. So we mainly discuss the case that
$G_b$ is connected.

The proof consists of three
parts. First, we show that for the class of bipartite graphs, Theorem~\ref{thm:whitney} holds without exception. Second, we will show how to construct a \emph{line expansion} $G_l$ from the bipartite representation $G_b$.
Third, we show how to recover the bipartite graph $G_b$ from $G_l$.

 First, for the exception in Whitney's theorem, it is obvious that $K_3$ (in Fig.~\ref{fig:appendix2}) cannot be the bipartite representation of any hypergraph. Therefore, 
for bipartite graphs, Theorem~\ref{thm:whitney} holds without exception.

(Injectivity) Second, according to Definition~\ref{def:linegraph}, the \emph{line expansion} $G_l$ of the hypergraph is equivalent to line graph of star expansion $G_s$, which is the line graph of bipartite representation $G_b$, i.e., $L(G_b)$. Also, Theorem~\ref{thm:whitney} guarantees that the topology 
of $L(G_b)$ is unique. The actual construction is given by Definition~\ref{def:linegraph} or Definition~\ref{def:lineexpansion}.

\begin{figure}[t]
	\centering
	\includegraphics[width=0.45\textwidth]{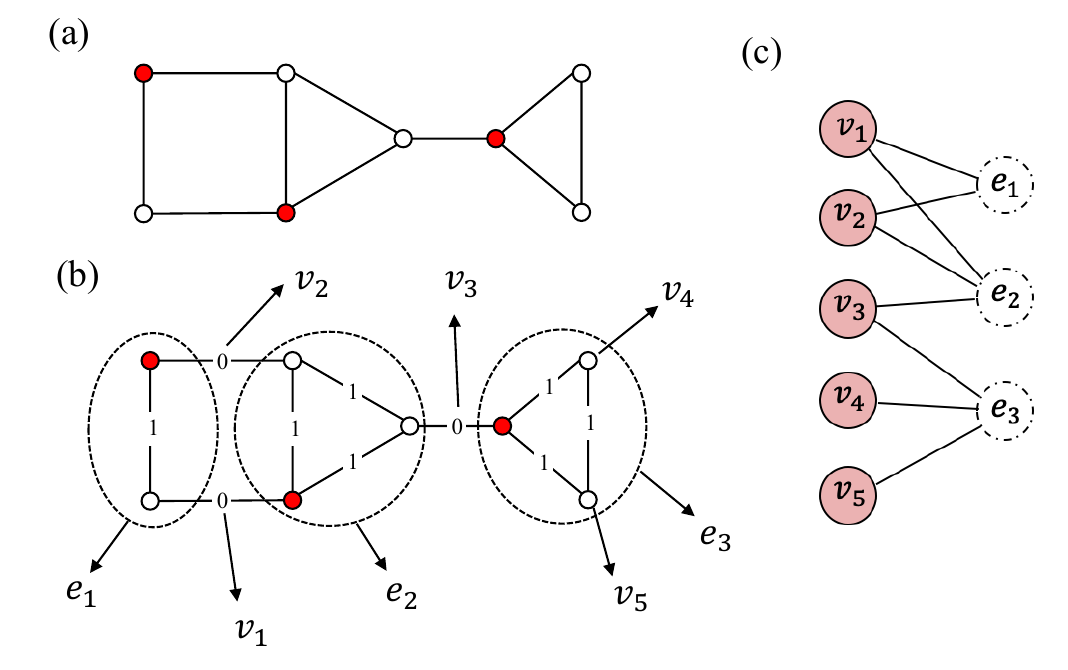}
	\vspace{-4mm}
	\caption{The construction from $G_l$ to $G_b$}
	\label{fig:appendix3}
\end{figure}

(Surjectivity) Third, given a line graph topology (of a bipartite graph), we know from Theorem~\ref{thm:whitney} immediately that the original bipartite structure is unique.
We now provide a construction from $G_l$ to $G_b$. Given a
line graph structure, we first find a maximum independent set (in Definition~\ref{def:maximummatching}) and color them in red (shown in Fig.~\ref{fig:appendix3} (a)). \cite{paschos2010combinatorial} proves that it could be found in polynomial time. 

% \begin{table*}[htbp] \small
% \centering
% \caption{Details of Matrices}
% 	{\begin{tabular}{ ccl} 
% 			\toprule
% 			\textbf{Matrix}  & \textbf{Size}  & \textbf{Detail} \\
% 			\midrule
% 			$H$ & $|V|\times|E|$ & $h(u,e)=1$ if and only if $u$ is incident to $e$. \\
% 			$D_v$ & $|V|\times |V|$ & $D_v(u,u)=\sum_eh(u,e)$, diagonal \\
% 			$D_e$ & $|E|\times |E|$ & $D_e(e',e')=\sum_eh(u,e')$, diagonal \\
% 			$P_v$ & $|V_l|\times |V|$ & $P_v(v_l, v')=1$ if and only if $v_l=(v',e)$ \\
% 			$P_e$ & $|V_l|\times |E|$ & $P_e(v_l, e')=1$ if and only if $v_l=(v,e')$ \\
% 			$H_r$ & $|V_l|\times (|V|+|E|)$ & see $P_v$ and $P_e$ \\
% 			{$A_l$} & {$|V_l|\times |V_l|$} & $A_l(u_l, v_l)=1$ for $u_l=(u,e)$ and $v_l=(u',e')$ \\
% 			&&if and only if $u=u'$ or $e=e'$ \\
% 			\bottomrule
% 	\end{tabular}}
% 	\label{tb:appendix4}
% \end{table*}

Since every vertex and hyperedge from $G_b$ spans a clique in $L(G_b)$. Let us think
about the node in this topology, it is potentially a vertex-hyperedge pair in the original hypergraph. Therefore, each node $(v, e)$ must be connected to exactly two cliques: one spanned by vertex $v$ and
one spanned by hyperedge $e$. Essentially, we try to project these cliques back to original vertex or hyperedges in $G_b$. In fact, for each colored node (three in Fig.~\ref{fig:appendix3} (a)), we choose one of two cliques connected to it so as to make sure: i) the selected cliques have no intersections (there is only two choices. In this case, choose cliques with $1$ on their edges or cliques with $0$
on their edges) and ii) the set of cliques cover all nodes in the topology, shown in Fig.~\ref{fig:appendix3} (b).

For any given line graph topology (of a bipartite graph), we could always find the set of cliques with $1$ on edges or the set of cliques with $0$ on edges that satisfies i) and ii), guaranteed by Definition~\ref{def:maximummatching}. Conceptually, due to the bipartite nature, one set will be the cliques
spanned by original hyperedges and another set will be the cliques spanned by original vertices. Either will work for us. Note that the set of cliques with $0$ on edges also includes two size-1 clique, denoted as $v_4$ and $v_5$ in Fig.~\ref{fig:appendix3} (b).
They seem to only connect to one clique  with $1$ on edges, i.e, $e_3$ clique, however, they are actually size-1 cliques spanned by original vertices which belongs
to only one hyperedge in $G_b$.

To construction of the bipartite representation $G_b$ is as follows: essentially each clique in the given topology will be either a vertex or a hyperedge in $G_b$. Suppose we have choose the set of cliques with $1$ on edges, we transform each selected clique as a hyperedge of  $G_b$. The vertex set is created two-folded: 
i) a clique with $0$ on its edges is a vertex in $G_b$ (In this case, we have three size-2 cliques with $0$ on their edges, i.e., $v_1$, $v_2$, $v_3$), and the vertex will be connected to the according hyperedges. For example, in Fig.~\ref{fig:appendix3} (c), $v_2$ will connected to $e_1$ and $e_2$ in $G_b$, because $v_2$ represents a size-2 clique with $0$ on its edges, $e_1$ and $e_2$ represent two selected cliques, and $v_2$ clique is connected to both $e_1$ clique and $e_2$ clique in this topology; ii) nodes only connected to one clique with $1$ on their edges are also designated to be vertices in $G_b$, and we connect them to the represented hyperedge. For example, two nodes denoted as $v_4$ and $v_5$ in Fig.~\ref{fig:appendix3} (b). They are indeed two size-1 clique with $0$ on their edges (it is not so obvious because size-1 clique has no edge). Indeed, these size-1 cliques
are spanned by vertices in original $G_b$ where they only connect to one hyperedge.

So far, we have reconstructed the bipartite representation $G_b$ in Fig.~\ref{fig:appendix3} (c) from a given line graph
structure in Fig.~\ref{fig:appendix3} (a). For those unconnected bipartite representation, we do the same reconstruction for each connected components. Thus,
we conclude the bijectivity of \emph{line expansion}.
\end{proof}

% \section{Details in Experiments} \label{details}
% \subsection{Simple Citation Network Classification}
% Following the same standard settings from \cite{yang2016revisiting} in this experiment, we treat links between nodes (documents) as undirected and only select 20 labeled data per class. For SpectralClustering, Node2Vec, DeepWalk and LINE, we first run them on the original graphs to get the representation of the nodes, and then this representation will be passed into a Multi-layer Perception (MLP) classifier with 32 hidden units. 

% To deploy our \emph{line expansion}, we transform (refer to Figure~\ref{fig:expansion}) each dataset into line domain by treating them as two-order hypergraphs, and then apply these five network representation methods.
